# Supplementary material for: Fidelity-Enhanced Variational Quantum Optimal Control
Source: arXiv:2501.17692 source file (2025-01-29)
Supplement: Supplementary file 1 [file Appendices.tex]

\documentclass[aps,pra,twocolumn,superscriptaddress]{revtex4-1}

\usepackage[english]{babel}
\usepackage{amsmath}
\usepackage{amsthm}
\usepackage{amssymb}
\usepackage{mathrsfs}
\usepackage{booktabs}
\usepackage{color}
\usepackage{hyperref}
\usepackage[ruled,vlined]{algorithm2e}
\usepackage{cases}
\usepackage{dblfloatfix}
\usepackage{multirow}
\hypersetup{
  colorlinks   = true,  %Colours links instead of ugly boxes
  urlcolor     = blue,  %Colour for external hyperlinks
  linkcolor    = blue,  %Colour of internal links
  citecolor    = red    %Colour of citations
}
\hyphenation{Fesh-bach}
\usepackage{mathtools}
\usepackage{natbib}
\usepackage{pgfplots}
\usepackage{subfigure}
\usepackage{url}

\newcommand{\rvline}{\hspace*{-\arraycolsep}\vline\hspace*{-\arraycolsep}}

\newcommand{\di}{{\rm d}}
\newcommand{\C}{{\sf C}}
\newcommand{\F}{{\sf F}}
\newcommand{\U}{{\sf U}}
\newcommand{\V}{{\sf V}}
\newcommand{\Y}{{\sf Y}}
\renewcommand{\L}{{\sf L}}
\renewcommand{\S}{{\sf S}}

\mathtoolsset{showonlyrefs}

\theoremstyle{definition}

\theoremstyle{remark}

\theoremstyle{plain}
\newtheorem*{theorem*}{Theorem}
\newtheorem*{lemma}{Lemma}

%Added
  % skewed hat on j for notation of Riccati-Bessel function

%Added
\usepackage{scalerel,stackengine}
\stackMath
\newcommand\reallywidehat[1]{%
\savestack{\tmpbox}{\stretchto{%
  \scaleto{%
    \scalerel*[\wi\di thof{\ensuremath{#1}}]{\kern-.6pt\bigwedge\kern-.6pt}%
    {\rule[-\textheight/2]{1ex}{\textheight}}%WIDTH-LIMITED BIG WEDGE
  }{\textheight}% 
}{0.5ex}}%
\stackon[1pt]{#1}{\tmpbox}%
}
\parskip 1ex

%Added
\usepackage{comment}
\usepackage{float}

\setlength\parindent{0pt}
\SetArgSty{textnormal}

\makeatletter

\makeatother

\begin{document}

\onecolumngrid

\appendix
\section{Formal derivation of the Stochastic Schr\"{o}dinger equation}
\label{app:ssederivation}
In this section, we follow the derivation of the SSE as in \cite{colorednoisepaper}. Consider an (OU) process $X(t)$ and operators $C,D$, and $R$ on the Hilbert space. The basic linear Schr\"{o}dinger equation with noise is given by
\begin{equation}
    \di \psi=(C+DX_t) \psi\, \di t+R \psi\, \di X_t.
\end{equation}
Using $\di X_t=-kX_t+\gamma \di W_t$, this can be rewritten as
\begin{equation}
    \di \psi=(C+X D-k X R) \psi\, \di t+ \gamma R \psi\, \di W_t.
\end{equation}
For normalization, $\di |\psi|^2=(\di \psi^\dagger)\psi+\psi^\dagger(\di\psi)+(\di\psi^\dagger)(\di\psi)=0$ is required at all times. Expanding this using Ito calculus ($\di t^2=0, \di W_t\di t=0, \di W_t^2=\di t)$ \cite{ito} gives
\begin{equation}
\di|\psi|^2=\psi^\dagger\left[C^{\dagger}+C+X_t\left(D^{\dagger}+D-k R-k R^{\dagger}\right)+\gamma^2 R^{\dagger} R\right]\psi \,\di t+\gamma \psi^\dagger (R^{\dagger}+R) \psi \,\di W_t=0.
\end{equation}
Thus, $C^\dagger+C+R^\dagger R=0$, $D^\dagger+D-kR-kR^\dagger=0$ and $R^\dagger+R=0$. One can choose $R=iS$ with $S=S^\dagger$ Hermitian. Furthermore, $C=-iH-\frac{1}{2}S^\dagger S=-iH-\frac{1}{2}S^2$, with $H=H^\dagger$ and $D=0$ to finally get the SSE for an (OU) process as
\begin{equation}
    \text{(OU)}:\quad \di \psi=-iH\psi \,\di t+i k X_t S\psi \,\di t-\frac{\gamma^2}{2} S^\dagger S \psi \,\di t - i\gamma S\psi \,\di W_t.\\
\end{equation}
Letting $k\rightarrow0$ results in the SSE for the (WN) process as 
\begin{equation}
    \text{(WN)}:\quad \di \psi=-iH\psi \,\di t-\frac{\gamma^2}{2} S^\dagger S \psi \,\di t - i\gamma S\psi \,\di W_t.\\
\end{equation}
Note that Ito calculus holds for any semimartingale \cite{ito}, and thus for general semimartingale noise we can write 
\begin{equation}
    \text{(SM)}:\quad \di \psi=-iH\psi \,\di t-\frac{1}{2}S^\dagger S \psi \,\di[X]_t - i S\psi \,\di X_t,\\
\end{equation}
where $[X]_t$ is the quadratic variation of the process \cite{quadvar}. By defining $\rho=\mathbb{E}[\psi\psi^\dagger]$ and noting that $\mathbb{E}[\di W_t]=0$
\begin{equation}
\begin{aligned}
\di \psi\psi^\dagger&=-i[H,\psi\psi^\dagger]\,\di t+(S\psi\psi^\dagger S^\dagger-\frac{1}{2}\{S^\dagger S,\psi \psi^\dagger\})\,\di [X]_t-i[S,\psi\psi^\dagger]\,\di X_t\\
\Rightarrow \partial_t\rho &=-i[H,\rho]+\gamma^2(S\rho^\dagger S^\dagger-\frac{1}{2}\{S^\dagger S,\rho\})-i[S,\mathbb{E}[\psi\psi^\dagger \,\di X_t]],
\end{aligned}
\end{equation}
which for white noise reduces to the Lindblad equation since $\mathbb{E}[\psi\psi^\dagger \di X_t]=\mathbb{E}[\psi\psi^\dagger \di W_t]=\mathbb{E}[\psi\psi^\dagger]\mathbb{E}[ \di W_t]=0$. Note that for general noise, there is no independence of the state and the noise increments (i.e. $\mathbb{E}[\psi\psi^\dagger \di X_t]\neq\mathbb{E}[\di X_t]\rho$), and we do not get the standard Lindblad equation.

\section{Ito's Isometry}
\label{app:itoiso}
We detail the approximation method for terms of the form $\mathbb{E}[X_t^2 \V]$ as described in Sec.~\ref{sec:odes}. The integral solution of the (OU) process \cite{ounoise} can be written as
\begin{equation}
    X_t=\int_0^t \gamma e^{k(s-t)} \di W_s.
\end{equation}
By positivity of $\V$
\begin{equation}
    \mathbb{E}[X_t^2 \V]=\mathbb{E}\left[\left(\int_0^t \gamma e^{k(s-t)} \di W_s\right)^2\V\right]=\mathbb{E}\left[\left(\int_0^t \gamma \sqrt{\V} e^{k(s-t)} \di W_s\right)^2\right].
\end{equation}
If $\V$ were to be adapted to the natural filtration of the Wiener process $W_t$, Ito's isometry \cite{itoisometry} can be used to write
\begin{equation}
    \mathbb{E}[X_t^2 \V]=\mathbb{E}\left[\int_0^t \gamma^2 \V e^{2k(s-t)} \di t\right]=\frac{\gamma^2}{2k}(1-e^{-2kt})\mathbb{E}[\V]=\mathbb{E}[X_t^2]\mathbb{E}[\V].
\end{equation}
However, $\V$ could for instance be the fidelity at time $t$ which is dependent on the Wiener process in the interval $[0,t]$. Therefore, Ito's isometry does not hold. Nevertheless, for small values of $t$, the $\V$ values are roughly equal to their respective initial values, and Ito's isometry can be used as an approximation.  

\section{Moment calculation}
\label{app:cosexp}
For the expectation and variance of the fidelity distributions, expressions for the expectations of terms $\cos(\alpha(X_t-X_0))$ for $\alpha>0$ have to be calculated (note that for square terms $\cos(x)^2=(\cos(2x)+1)/2$). To do so, the cosines are expanded into their power series representation, and both linearity and conditional expectations are used to get
\begin{equation}
\label{eq:expcos}
    \mathbb{E}[\cos(\alpha(X_t-X_0))]=\sum_{n=0}^\infty \frac{(-1)^n}{2n!}\alpha^{2n}\mathbb{E}\big[\mathbb{E}[(X_t-X_0)^{2n}|X_0]\big].
\end{equation}

The (OU) process, by Ito's formula \cite{itoisometry}, can be shown to obey
\begin{equation}
\label{eq:difou}
    \di X_t^{n}=-nkX^{n}\di t+n\gamma X^{n-1}\di W_t+\frac{1}{2}(n^2-n)\gamma^2X^{n-2}\di t, \quad X^n(0)\sim X_0^n,\quad \forall n\in \mathbb{N}.
\end{equation}

\subsection*{Calibrated initial data $X_0=0$}

For calibrated initial data (e.g. $X_0=0$), it is easily proven by induction that
\begin{equation}
\label{eq:expcalibrated}
    \mathbb{E}\big[\mathbb{E}[(X_t-X_0)^{2n}|X_0]\big]=\mathbb{E}[X_t^{2n}]=\frac{\Gamma \left(n+\frac{1}{2}\right) }{\sqrt{\pi }}\left(\frac{2\gamma^{2}}{k}e^{-k  t} \sinh (k t)\right)^n.
\end{equation}
where $\Gamma$ is the gamma function. Resulting from Eq.~\eqref{eq:expcos} in
\begin{equation}
    \mathbb{E}[\cos(\alpha(X_t-X_0))]=\exp\left(-\alpha^2\frac{\gamma^2}{2k} e^{-k t} \sinh(kt) \right).
\end{equation}

\subsection*{Stationary initial data $X_0\sim \gamma\mathcal{N}/\sqrt{2k}$}

For stationary initial data, a slightly more involved approach is necessary, where the binomial theorem is employed to get
\begin{equation}
\label{eq:binomial}
    \mathbb{E}[(X_t-X_0)^{2n}|X_0]=\sum_{m=0}^{2n}\binom{2n}{m}(-1)^{2n-m}X_0^{2n-m}\mathbb{E}[X_t^m|X_0].
\end{equation}
From the differential equations in Eq.~\eqref{eq:difou}
\begin{equation}
    d\mathbb{E}[X_t^m|X_0]=-mk\mathbb{E}[X_t^m|X_0]\di t+\frac{1}{2}(m^2-m)\gamma^2\mathbb{E}[X_t^{m-2}|X_0]\di t,
\end{equation}
with initial conditions $\mathbb{E}[X_t^0|X_0]=1,\, \mathbb{E}[X_t^1|X_0]=X_0e^{-kt}.$ This can be shown to have the solution
\begin{equation}
\label{eq:expxtm}
\begin{aligned}
\mathbb{E}[X_t^m|X_0]&=\begin{cases}e^{-2wkt}(2k)^{-w}
 \sum_{l=0}^{w}a[l, w](e^{2kt}-1)^{w - l}\gamma^{2(w - l)}k^l
   X_0^{2l},\quad\,\,\,\,\, w=m/2,\qquad \,\,\,\text{ for } m \text{ even}
   \\e^{-(2w+1)kt}(2k)^{-w}
   \sum_{l=0}^{w}b[l, w](e^{2kt}-1)^{w - l}\gamma^{2 (w - l)}k^l
     X_0^{2 l+1}, \quad w=(m-1)/2, \text{ for } m \text{ odd}
\end{cases},\\
&a[l,w] := 2^l\prod_{q=l+1}^w\frac{q (2 q - 1)}{q - l}
   ,\quad b[l,w] := 2^l\prod_{q=l}^{w-1}\frac{(1 + q) (3 + 2 q)}{(q - l + 1)}.
\end{aligned}
\end{equation}

For verification, the expressions for $\mathbb{E}[X_t^{2m}]$ in the case of calibrated initial data (Eq.~\eqref{eq:expcalibrated}) are retrieved when taking $X_0=0$. Using conditional expectation on Eq.~\eqref{eq:binomial} gives

\begin{equation}
\label{eq:expxtmx0}
    \mathbb{E}\big[\mathbb{E}[(X_t-X_0)^{2n}|X_0]\big]=\sum_{m=0}^{2n}\binom{2n}{m}(-1)^{2n-m}\mathbb{E}[X_0^{2n-m}\mathbb{E}[X_t^m|X_0]].
\end{equation}
Furthermore, the normal distribution of $X_0$ gives
\begin{equation}
\label{eq:normaldis}
    \mathbb{E}[X_0^q]=\begin{cases} \left(\frac{\gamma}{\sqrt{2k}}\right)^q(q-1)!!, \quad q \text{ even }
   \\0, \quad q \text{ odd }.
\end{cases}
\end{equation}
Combining Eq.~\eqref{eq:expxtm} and Eq.~\eqref{eq:normaldis}, and filling into Eq.~\eqref{eq:expxtmx0} gives
\begin{equation}
    \mathbb{E}[\mathbb{E}[(X_t-X_0)^{2n}|X_0]]=(2 n - 1)!!\left(\frac{\gamma^2}{k}e^{-kt}(e^{kt}-1)\right)^n,
\end{equation}
which, when used in Eq.~\eqref{eq:expcos}, results in
\begin{equation}
    \mathbb{E}[\cos(\alpha(X_t-X_0))]=\exp\left(-\alpha^2 \frac{\gamma^2}{2k} e^{-k t} (e^{k t}-1)\right).
\end{equation}

\section{Multi-qubit noise}
\label{app:multiq}
This section proves a lemma regarding the factoring of fidelity distributions of $n$-qubit systems, which have a product initial state and evolve under the same noise source.
\begin{lemma}[Factoring fidelity for pure states]
Let the state $\psi_{(n)}$ of a $n$-qubit system evolve according to
\begin{equation}
    \di \psi_{(n)}=-iH_n\psi_{(n)}\di t-\frac{1}{2}S_n^2\psi_{(n)}\di [X]_t-iS_n\psi_{(n)} \di X_t,\quad \psi_{(n)}(0)=\bigotimes_{j=1}^n \psi_{j0},
\end{equation}
where the Hamiltonian $H_n$ and the noise operator $S_n$ take the sum form
\begin{equation}
\begin{aligned}
    H_n&=\sum_{j=1}^n A_j,\quad A_j=I^{\otimes (j-1)}\otimes \tilde{A}_j \otimes I^{\otimes (n-j)},\quad \tilde{A_j}=\tilde{A_j}^\dagger,\\
    S_n&=\sum_{j=1}^n Q_j,\quad Q_j=I^{\otimes (j-1)}\otimes \tilde{Q}_j \otimes I^{\otimes (n-j)},\quad \tilde{Q_j}=\tilde{Q_j}^\dagger.
\end{aligned}
\end{equation}
Let $\phi_{(n)}$ be the noiseless target state. Then 
\[
	|\phi_{(n)}^\dagger \psi_{(n)}|^2=\prod_{j=1}^n |\phi_j^\dagger \psi_j|^2,
\] where $\psi_j$ is a 1-qubit state evolving according to the SSE
\begin{equation}
        \di \psi_j=-i\tilde{A}_j\psi_j\,\di t-\frac{1}{2} \tilde{Q}_j^2\psi_j \,\di [X]_t-i \tilde{Q}_j \psi_j \,\di X_t , \quad \psi_j(0)=\psi_{j0},
\end{equation}
and $\phi_j$ is its corresponding noiseless target state. 
\end{lemma}

\begin{proof}
Squaring  $S_n$, we find
\begin{equation}
    S_n^2=\sum_{j=1}^n Q_j^2+\sum_{j=1}^n\sum_{k\neq j}^n Q_{jk},\quad Q_{jk}=I^{\otimes (j-1)}\otimes \tilde{Q}_j \otimes I^{\otimes (k-j-1)} \otimes \tilde{Q}_k \otimes I^{\otimes (n-k)}.
\end{equation}
By induction we prove the $\psi_{(n)}=\bigotimes_{j=1}^n \psi_j$. 

\smallskip

This holds trivially for $n=1$. Now, assume the statement holds for $n$. Then for $n+1$, we use It\^o's formula to obtain
\begin{equation}
\begin{aligned}
    \di\bigotimes_{j=1}^{n+1} \psi_j
    =-iH_{n+1}\bigotimes_{j=1}^{n+1} \psi_j\,\di t-iS_{n+1}\bigotimes_{j=1}^{n+1} \psi_j\,\di X_t-\frac{1}{2}S_{n+1}\bigotimes_{j=1}^{n+1} \psi_j \,\di [X]_t.
\end{aligned}
\end{equation}
As we have equal initial conditions, we indeed find $\psi_{(n+1)}=\bigotimes_{j=1}^{n+1} \psi_j$ for all $n\in\mathbb{N}$.

\smallskip

Analogously, we find $\phi_{(n)}=\bigotimes_{j=1}^{n} \phi_j$. For the fidelity, we then deduce
\begin{equation}
    |\phi_{(n)}^\dagger \psi_{(n)}|^2=\phi_{(n)}^\dagger \psi_{(n)}\psi_{(n)}^\dagger\phi_{(n)}=\left(\bigotimes_{j=1}^{n} \phi_j^\dagger \bigotimes_{j=1}^{n} \psi_j\right)\left(\bigotimes_{j=1}^{n} \psi_j^\dagger \bigotimes_{j=1}^{n} \phi_j\right)=\prod_{j=1}^n |\phi_j^\dagger\psi_j|^2. 
\end{equation}
\end{proof}

Note that these results do not only hold for qubits, but for any finite ensemble of finite dimensional quantum systems.

\section{Stochastic Integration}
\label{app:stochint}
Numerical verification of the analytic results is performed using stochastic integration. To solve for the noise and state simultaneously, we define $\Y:=(\psi,X)$. For the (OU) process, this gives the differential equation
\begin{equation}
    \di \Y=a(\Y)\,\di t+b(\Y)\,\di W_t,\quad a(\Y)=
\begin{pmatrix}
-iH+ikXS-\frac{\gamma^2}{2}S^\dagger S
  & \rvline & \mathbf{0} \\
\hline
  \mathbf{0}^\text{T} & \rvline &
-k
\end{pmatrix}\Y,\quad b(\Y)=\begin{pmatrix}
-i\gamma S
  & \rvline & \mathbf{0} \\
\hline
  \mathbf{0}^\text{T} & \rvline &
\frac{1}{X}
\end{pmatrix}\Y.
\end{equation}
These equations can be solved discretely over time steps $\Delta t$ using a numerical integration scheme. One possible scheme is the explicit (weak) first-order Euler-Maruyama scheme \cite{stochasticintegration1} as
\begin{equation}
    \Y_{n+1}=\Y_n+a(\Y_n)\Delta t+b(\Y_n)\mathcal{N}\sqrt{\Delta t},
\end{equation}
where $\mathcal{N}$ is a standard normal distribution. Throughout this work, convergences issues persisted using stochastic integration schemes for (OU) noise at higher evolution times, likely due to the non-Lipschitz $1/X$ dependence \cite{platen} and possibly the non-Euclidean space in which the states live. These convergence issues are absent for white noise and always occur below fidelities of $F=0.95$, which is not a relevant regime for pragmatic quantum computing and therefore not a deliberating issue. We have found that these issues are mitigated (but not resolved) when using a higher-order scheme such as the explicit (weak) second-order scheme due to Platen \cite{stochasticintegration2,platen}, which is used throughout this work. This scheme is given by 
$$
\begin{aligned}
& \Y_{n+1}=\Y_n+\frac{1}{2}\big(a(\bar{\Upsilon})+a(\Y_n)\big) \Delta t+\frac{1}{4}\big(b\left(\bar{\Upsilon}^{+}\right)+b\left(\bar{\Upsilon}^{-}\right)+2 b(\Y_n)\big) \mathcal{N}\sqrt{\Delta t} +\frac{1}{4}\big(b(\tilde{\Upsilon}^{+})-b(\widetilde{\Upsilon}^{-})\big)\left(\mathcal{N}^2-1\right) \sqrt{\Delta t}, 
\end{aligned}
$$
with supporting values $\bar{\Upsilon}=\Y_n+a(\Y_n) \Delta t+b(\Y_n) \mathcal{N}\sqrt{\Delta t}$ and $\bar{\Upsilon}^{ \pm}=\Y_n+a(\Y_n) \Delta t \pm b(\Y_n) \sqrt{\Delta t}$.

\section{Second-order Pauli Approximation}
\label{app:secondorder}

For the second-order results as in Fig.~\ref{fig:orderofapprox},  the closed system for the vector $\V$
\begin{equation}
\begin{aligned}
    \V=\bigg[|\phi^\dagger\psi|^2,|\phi^\dagger S\psi|^2,X(t)(\phi^\dagger S\psi\psi^\dagger \phi-\phi^\dagger \psi\psi^\dagger S\phi), X^2(t)|\phi^\dagger\psi|^2,X^2(t)|\phi^\dagger S\psi|^2,X^3(t)(\phi^\dagger S\psi\psi^\dagger \phi-\phi^\dagger \psi\psi^\dagger S\phi)\bigg],
\end{aligned}
\end{equation}
is found to be
\begin{equation}
\dot{\V}=\left[
\begin{array}{cccccc}
 -\gamma^2 & \gamma^2 & ik & 0 & 0 & 0 \\
 \gamma^2 & - \gamma^2 & -ik & 0 & 0 & 0 \\
 -2i\gamma^2 & 2i\gamma^2 & -(k+2 \gamma^2) & 2ik & -2ik & 0 \\
 \gamma^2 & 0 & -2 i\gamma^2 & -(2k+\gamma^2) & \gamma^2 & i k \\
 0 & \gamma^2 & 2 i\gamma^2 & \gamma^2 & -(2k+\gamma^2) &  -i k \\
 0 & 0 & 2\gamma^2 & 2i(k\mathbb{E}[X_t^2]-2\gamma^2) & -2i(k\mathbb{E}[X_t^2]-2\gamma^2) & -(3k+2 \gamma^2) \\
\end{array}
\right]\V, \quad \V(0)=\left[
\begin{array}{c}
 1  \\
 \S_0^2 \\
 0\\
 0 \\
 0\\
 0 
\end{array}
\right],
\end{equation}
with $\S_0=\phi_0^\dagger S\phi_0$. This system is solved numerically to retrieve the expectation value of the fidelity.

\section{Non-commuting}
For the non-commuting system we consider $H=\alpha \sigma_1$, $S=\sigma_2$, giving $[H,S]=2i\alpha\sigma_3$, where $\{\sigma_1,\sigma_2,\sigma_3\}$ can be any cyclic permutation of $\{\sigma_X,\sigma_Y,\sigma_Z\}$. The group structure of the Pauli matrices allows us to close the system of ODEs for the vector
\label{app:noncommute}
\begin{equation}
\begin{aligned}
\V = \begin{bmatrix}
	\F \\ |\phi^\dag \sigma_1 \psi|^2 \\ |\phi^\dag \sigma_2 \psi|^2 \\ |\phi^\dag \sigma_3 \psi|^2 \\ i(\phi^\dag \sigma_1 \psi \psi^\dag \phi - \phi^\dag \psi \psi^\dag \sigma_1 \phi) \\ i(\phi^\dag \sigma_2 \psi \psi^\dag \phi - \phi^\dag \psi \psi^\dag \sigma_2 \phi) \\ i(\phi^\dag \sigma_3 \psi \psi^\dag \phi - \phi^\dag \psi \psi^\dag \sigma_3 \phi) \\ \phi^\dag \sigma_2 \psi \psi^\dag \sigma_1 \phi + \phi^\dag \sigma_1 \psi \psi^\dag \sigma_2 \phi \\ \phi^\dag \sigma_3 \psi \psi^\dag \sigma_1 \phi + \phi^\dag \sigma_1 \psi \psi^\dag \sigma_3 \phi \\ \phi^\dag \sigma_3 \psi \psi^\dag \sigma_2 \phi + \phi^\dag \sigma_2 \psi \psi^\dag \sigma_3 \phi
\end{bmatrix}\in\mathbb{R}^{10}.
\end{aligned}
\end{equation}
We find that the matrix $A$ splits in a commutator part $A_c$ and a noise part $B^2$, resulting in the system
\begin{equation}
    \di \V=\alpha A_c \V\,\di t+\frac{1}{2}\gamma^2 B^2\V\,\di t+ B\V\,\di X_t,
\end{equation}
with
\begin{equation}
A_c = 
    \begin{pmatrix}
         0 & 0 & 0 &  0 & 0 & 0 & 0 & 0 & 0 & 0 \\
         0 & 0 & 0 &  0 & 0 & 0 & 0 & 0 & 0 & 0 \\
         0 & 0 & 0 &  0 & 0 & 0 & 0 & 0 & 0 & -2 \\
         0 & 0 & 0 &  0 & 0 & 0 & 0 & 0 & 0 & 2 \\
         0 & 0 & 0 &  0 & 0 & 0 & 0 & 0 & 0 & 0 \\
         0 & 0 & 0 &  0 & 0 & 0 & -2 & 0 & 0 & 0 \\
         0 & 0 & 0 &  0 & 0 & 2 & 0 & 0 & 0 & 0 \\
         0 & 0 & 0 &  0 & 0 & 0 & 0 & 0 & -2 & 0 \\
         0 & 0 & 0 &  0 & 0 & 0 & 0 & 2 & 0 & 0 \\
         0 & 0 & 4 & -4 & 0 & 0 & 0 & 0 & 0 & 0 \\
    \end{pmatrix},\qquad
B =
    \begin{pmatrix}
        0 & 0 & 0 & 0 & 0 & -1 & 0 & 0 & 0 & 0 \\
         0 & 0 & 0 & 0 & 0 & 0 & 0 & 0 & 1 & 0 \\
         0 & 0 & 0 & 0 & 0 & 1 & 0 & 0 & 0 & 0 \\
         0 & 0 & 0 & 0 & 0 & 0 & 0 & 0 & -1 & 0 \\
         0 & 0 & 0 & 0 & 0 & 0 & 1 & -1 & 0 & 0 \\
         2 & 0 & -2 & 0 & 0 & 0 & 0 & 0 & 0 & 0 \\
         0 & 0 & 0 & 0 & -1 & 0 & 0 & 0 & 0 & -1 \\
         0 & 0 & 0 & 0 & 1 & 0 & 0 & 0 & 0 & 1 \\
         0 & -2 & 0 & 2 & 0 & 0 & 0 & 0 & 0 & 0 \\
         0 & 0 & 0 & 0 & 0 & 0 & 1 & -1 & 0 & 0 \\
    \end{pmatrix}.
%    A_2 =
%    \begin{pmatrix}
%        -1 & 0 & 1 & 0 & 0 & 0 & 0 & 0 & 0 & 0 \\
%         0 & -1 & 0 & 1 & 0 & 0 & 0 & 0 & 0 & 0 \\
%         1 & 0 & -1 & 0 & 0 & 0 & 0 & 0 & 0 & 0 \\
%         0 & 1 & 0 & -1 & 0 & 0 & 0 & 0 & 0 & 0 \\
%         0 & 0 & 0 & 0 & -1 & 0 & 0 & 0 & 0 & -1 \\
%         0 & 0 & 0 & 0 & 0 & -2 & 0 & 0 & 0 & 0 \\
%         0 & 0 & 0 & 0 & 0 & 0 & -1 & 1 & 0 & 0 \\
%         0 & 0 & 0 & 0 & 0 & 0 & 1 & -1 & 0 & 0 \\
%         0 & 0 & 0 & 0 & 0 & 0 & 0 & 0 & -2 & 0 \\
%         0 & 0 & 0 & 0 & -1 & 0 & 0 & 0 & 0 & -1 \\
%    \end{pmatrix},
\end{equation}
%\begin{equation}
%B =
%    \begin{pmatrix}
%        0 & 0 & 0 & 0 & 0 & -1 & 0 & 0 & 0 & 0 \\
%         0 & 0 & 0 & 0 & 0 & 0 & 0 & 0 & 1 & 0 \\
%         0 & 0 & 0 & 0 & 0 & 1 & 0 & 0 & 0 & 0 \\
%         0 & 0 & 0 & 0 & 0 & 0 & 0 & 0 & -1 & 0 \\
%         0 & 0 & 0 & 0 & 0 & 0 & 1 & -1 & 0 & 0 \\
%         2 & 0 & -2 & 0 & 0 & 0 & 0 & 0 & 0 & 0 \\
%         0 & 0 & 0 & 0 & -1 & 0 & 0 & 0 & 0 & -1 \\
%         0 & 0 & 0 & 0 & 1 & 0 & 0 & 0 & 0 & 1 \\
%         0 & -2 & 0 & 2 & 0 & 0 & 0 & 0 & 0 & 0 \\
%         0 & 0 & 0 & 0 & 0 & 0 & 1 & -1 & 0 & 0 \\
%    \end{pmatrix}.
%\end{equation}
Solving this system as in Sec.~\ref{sec:odes} is not possible since $[A_c,B]\ne 0$. However, a perturbation technique can be used when the Hamiltonian strength is much larger than the noise, i.e.\ $\varepsilon^2 :=\gamma^2/\alpha\ll 1$, which holds for many realistic systems. Rescaling time $\widehat t = t/\alpha$, we obtain a rescaled system of equations for $\widehat\V= \V_{t/\alpha}$ and $\widehat X = X_{t/\alpha}$,
\begin{equation}
    \di \widehat\V= A_c \widehat\V\,\di \widehat t + \frac{1}{2}\varepsilon^2 B^2\widehat\V\,\di \widehat t + B\widehat \V\,\di \widehat X_t,
\end{equation}
where $\widehat X$ has the quadratic variation $[\widehat X]_{\widehat t} = \varepsilon^2 \widehat t$. \\

In the following, we assume w.l.o.g.\ that $\alpha=1$ and $\gamma^2\ll 1$. Otherwise, we simply rescale time as above and write $\V$ in place of $\widehat\V$. Setting $\U:=\exp(-A_c t)\V$ to get
\begin{equation}
\label{eq:gho}
    \di\U=\frac{1}{2}\gamma^2 D^2(t)\U\, \di t+D(t)\U\, \di X_t,
\end{equation}
with 
\begin{equation}
D(t)=\exp(-A_c t)B\exp(A_c t)=\cos(2 t) B-\frac{1}{2}\sin(2 t)[A_c,B],
\end{equation}
where the second equality can be established according to a generalized harmonic oscillator \cite{introquantcalc}. Although \eqref{eq:gho} cannot be solved explicitly, an approximation to its solution can be found via the stochastic Magnus expansion \cite{stochasticmagnus}, which states that 
\begin{equation}
    \U=\exp(\L)=\exp\left(\sum_{n,r} \gamma^{2n-r}\L^{(r,n-r)}\right),
\end{equation}
where $\L^{(r,n-r)}$ are the expansion terms up to order $\gamma^2$ in $\L$. For general processes we find
\begin{equation}
    \U_t=\exp\left(\int_{0}^t D(s)\,\di X_s+O(\gamma^3)\right),
\end{equation}
which, for white noise, (WN) gives 
\begin{equation}
    \mathbb{E}[\U_t]\approx\exp\left(\frac{\gamma^2}{2}\int_{0}^t D^2(s)\,ds\right).
\end{equation}
For the fidelity under white noise, we obtain the approximation
\begin{equation}
    \F_t=\mathbb{E}[\U_t]\approx\frac{1}{2}+\frac{1}{2} \\C_1^2 e^{-2 \gamma^2 t}+\frac{1}{2} e^{-\gamma^2 t} \Bigl(\sinh (u) ((\C_2^2-\C_3^2) \cos (2a t)-2 \C_2 \C_3
   \sin (2a t))+\left(\C_2^2+\C_3^2\right) \cosh (u)\Bigr).
\end{equation}
% with $u=\gamma^2\sin(2at)/2a$. 
For the (OU) process with $k>0$, the exponential can not be expressed analytically. Instead, one could approximate it by expanding the exponential up to the second order to find

\begin{align*}
    \mathbb{E}[\U_t] &\approx I+\frac{\gamma^2}{2}\int_{0}^t  D^2(s) ds \\
    &\qquad - \frac{\gamma^2}{2} k\int_0^t \left\{e^{-ks} D(s),\int_{0}^{s}e^{ks'}D(s') ds' \right\}ds+\frac{\gamma^2}{4}k\int_{0}^t \left\{e^{-2ks}D(s),\int_{0}^s e^{2ks'}D(s')ds'\right\}ds.
\end{align*}

\bibliographystyle{apsrev4-1}
\bibliography{Bibliography.bib}

\end{document}
